# Supplementary material for: DiffSDA: Unsupervised Diffusion Sequential Disentanglement Across Modalities
Source: arXiv:2510.05717 source file (2025-10-07)

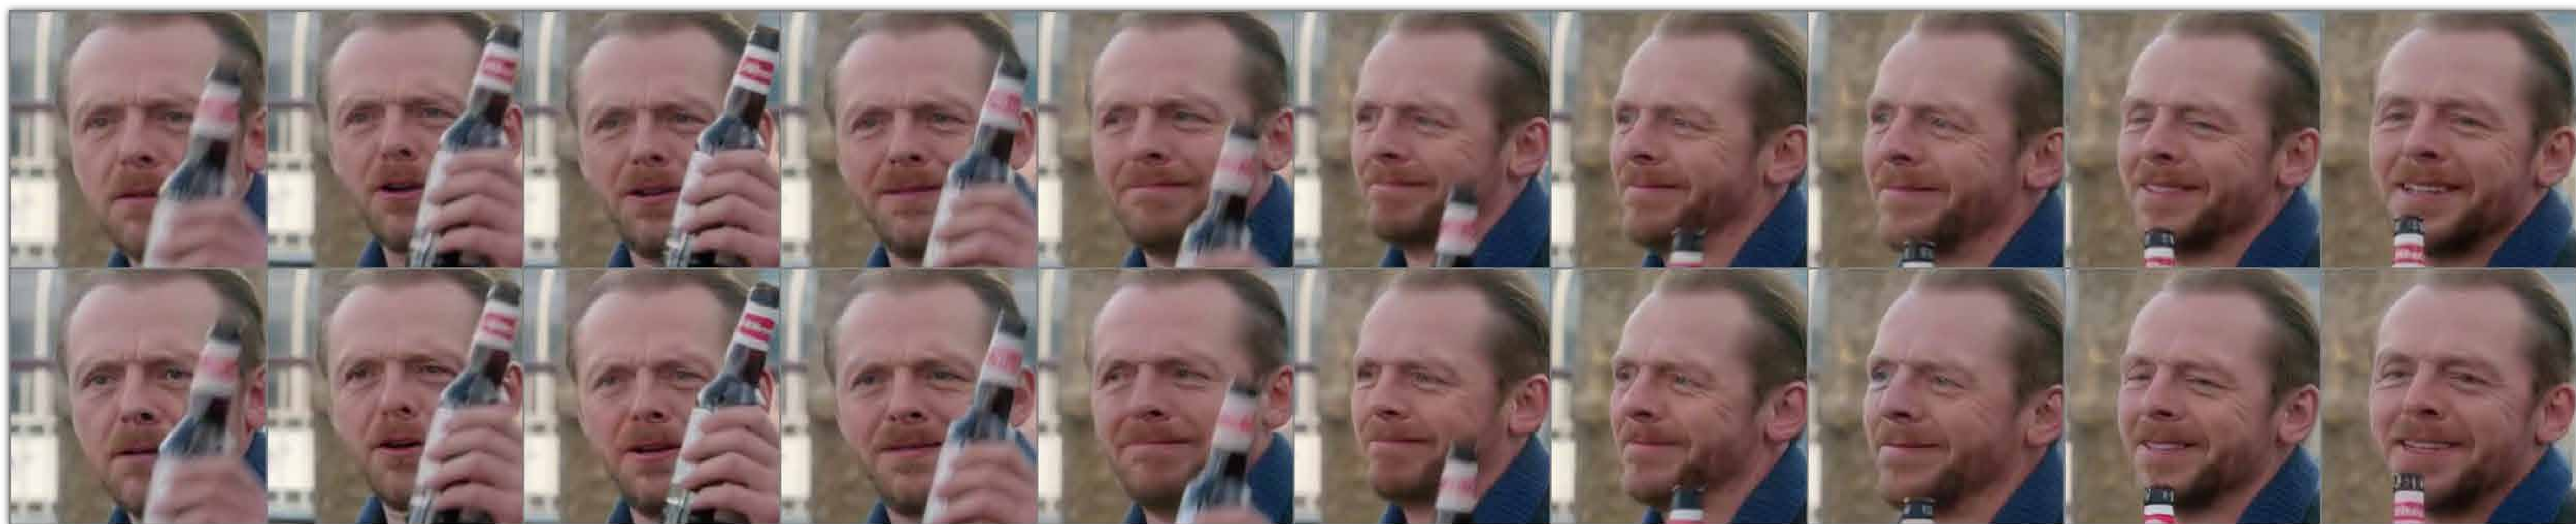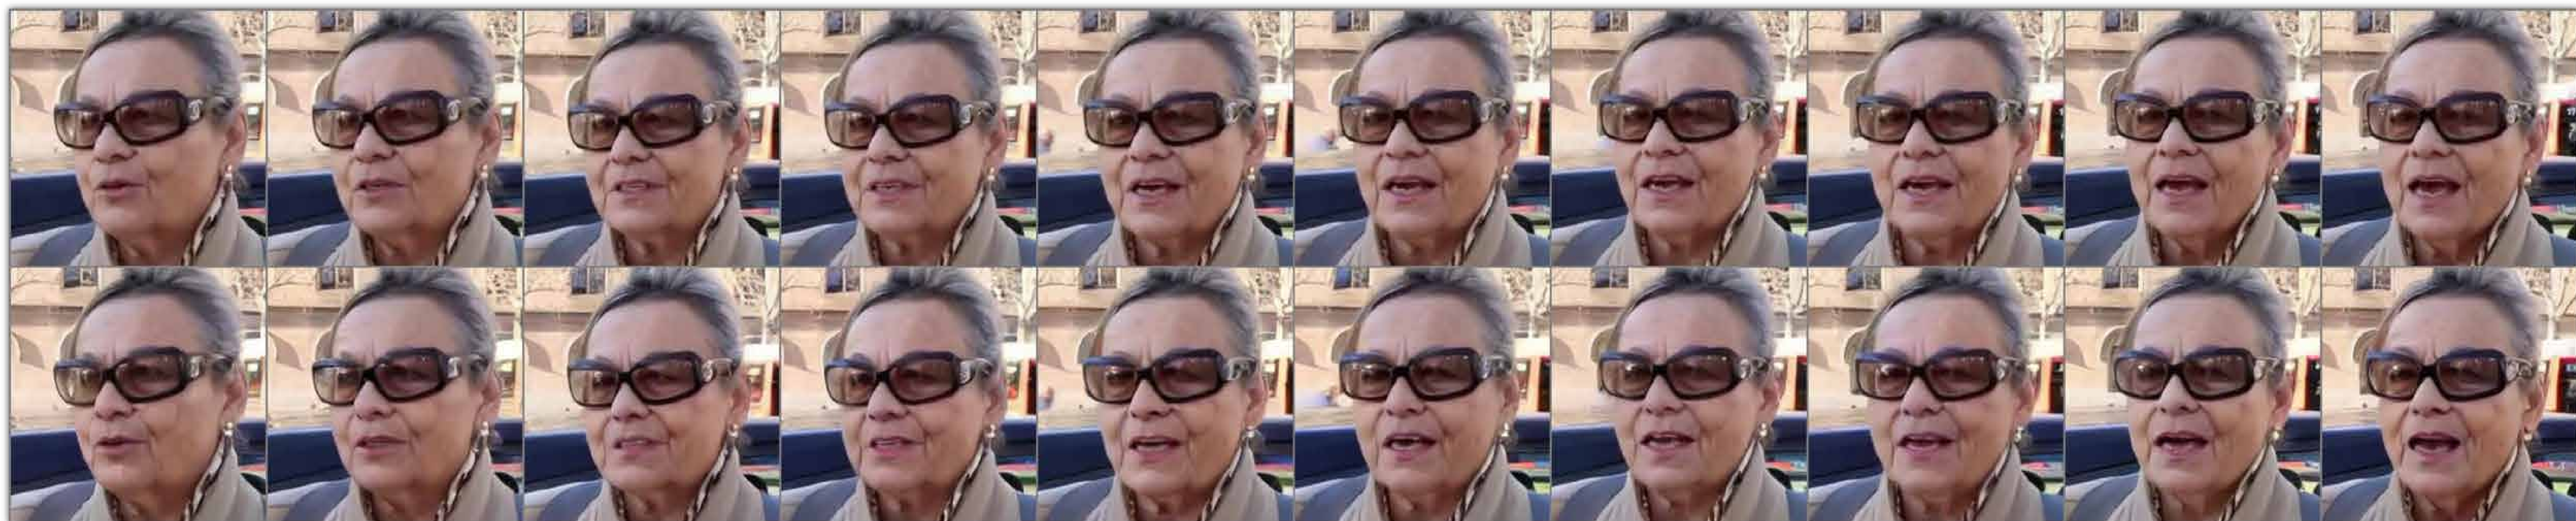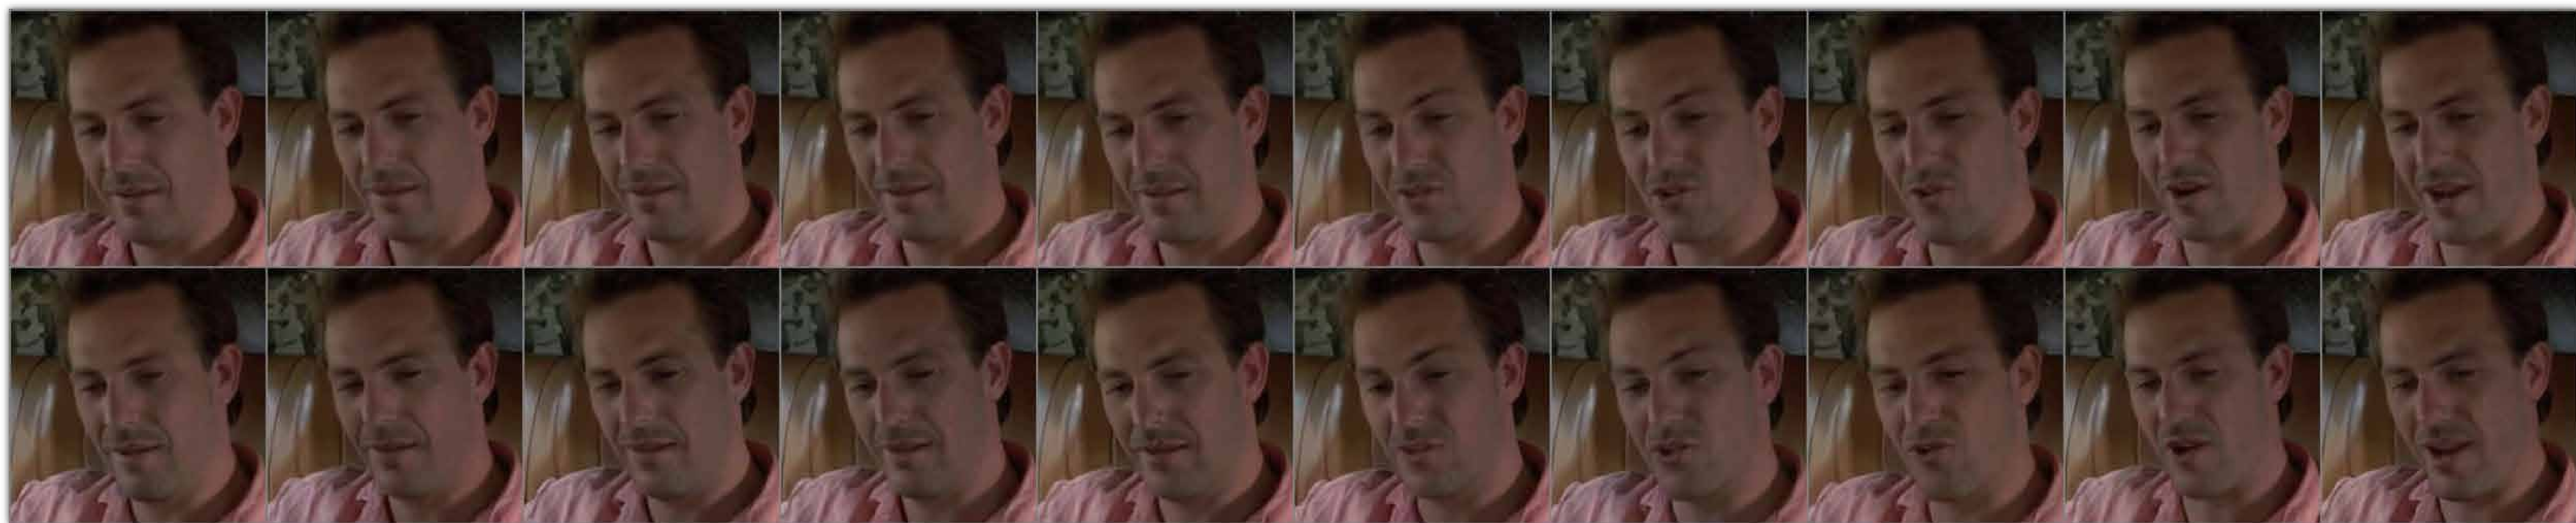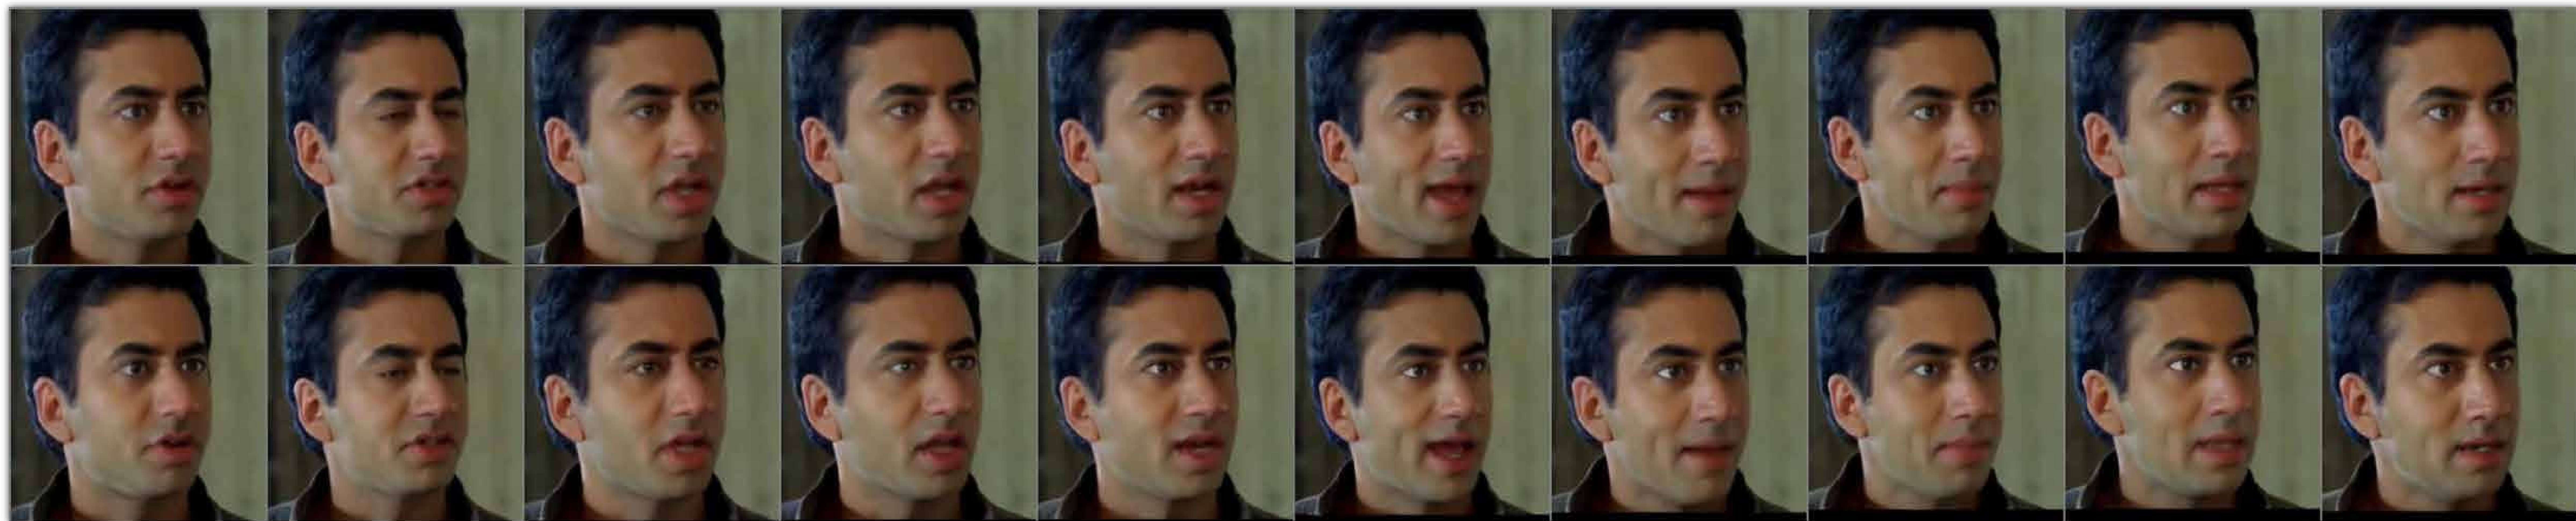



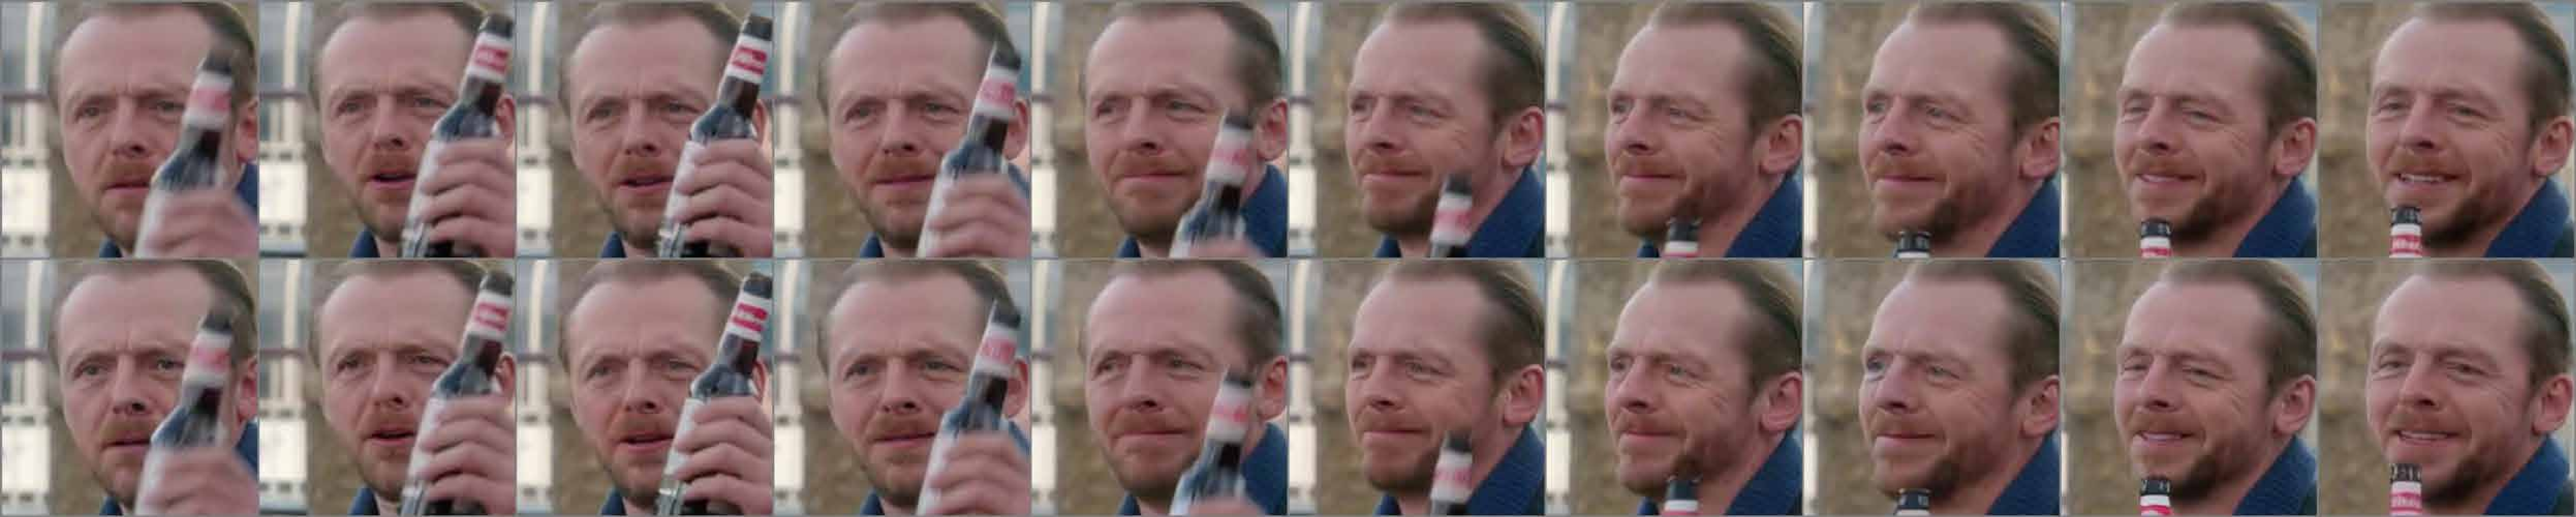

Supplement: Supplementary file 1 [file recon_sampels_celebv_app_lr2.pdf]
